# Supplementary material for: Ultrafast Electron Diffuse Scattering as a Tool for Studying Phonon Transport: Phonon Hydrodynamics and Second Sound Oscillations
Source: arXiv:2310.18793 ancillary file (2024-02-28)
Supplement: Supplementary file 1 [file supplement.pdf]

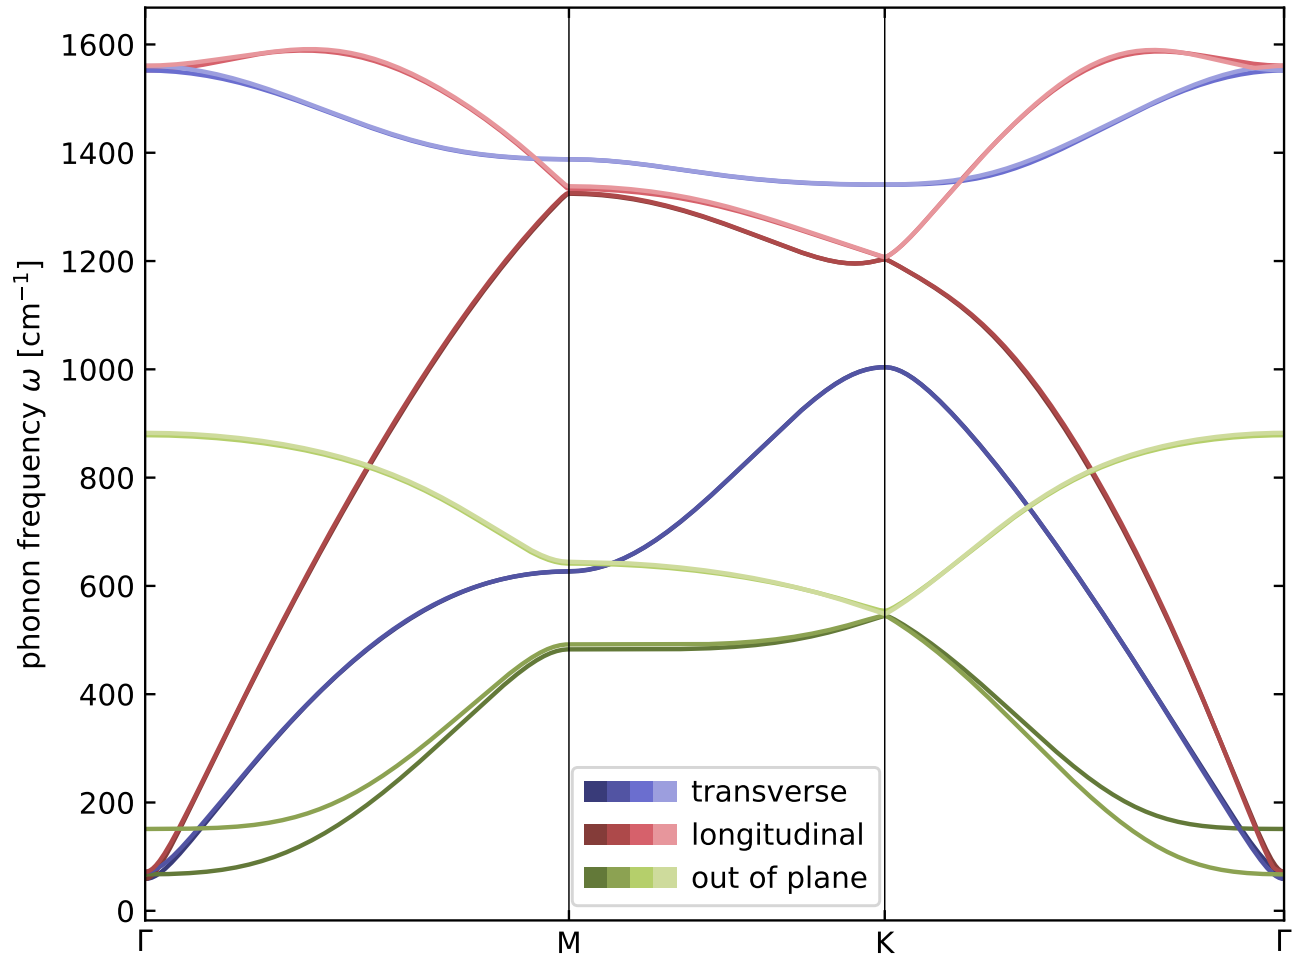

FIG. 1. Phonon band structure of graphite at 100 K following the path  $\overline{\Gamma\text{MK}\Gamma}$ . The four transverse modes (one acoustic, three optical) are depicted in blue, the four longitudinal ones in red and the out of plane modes in green.

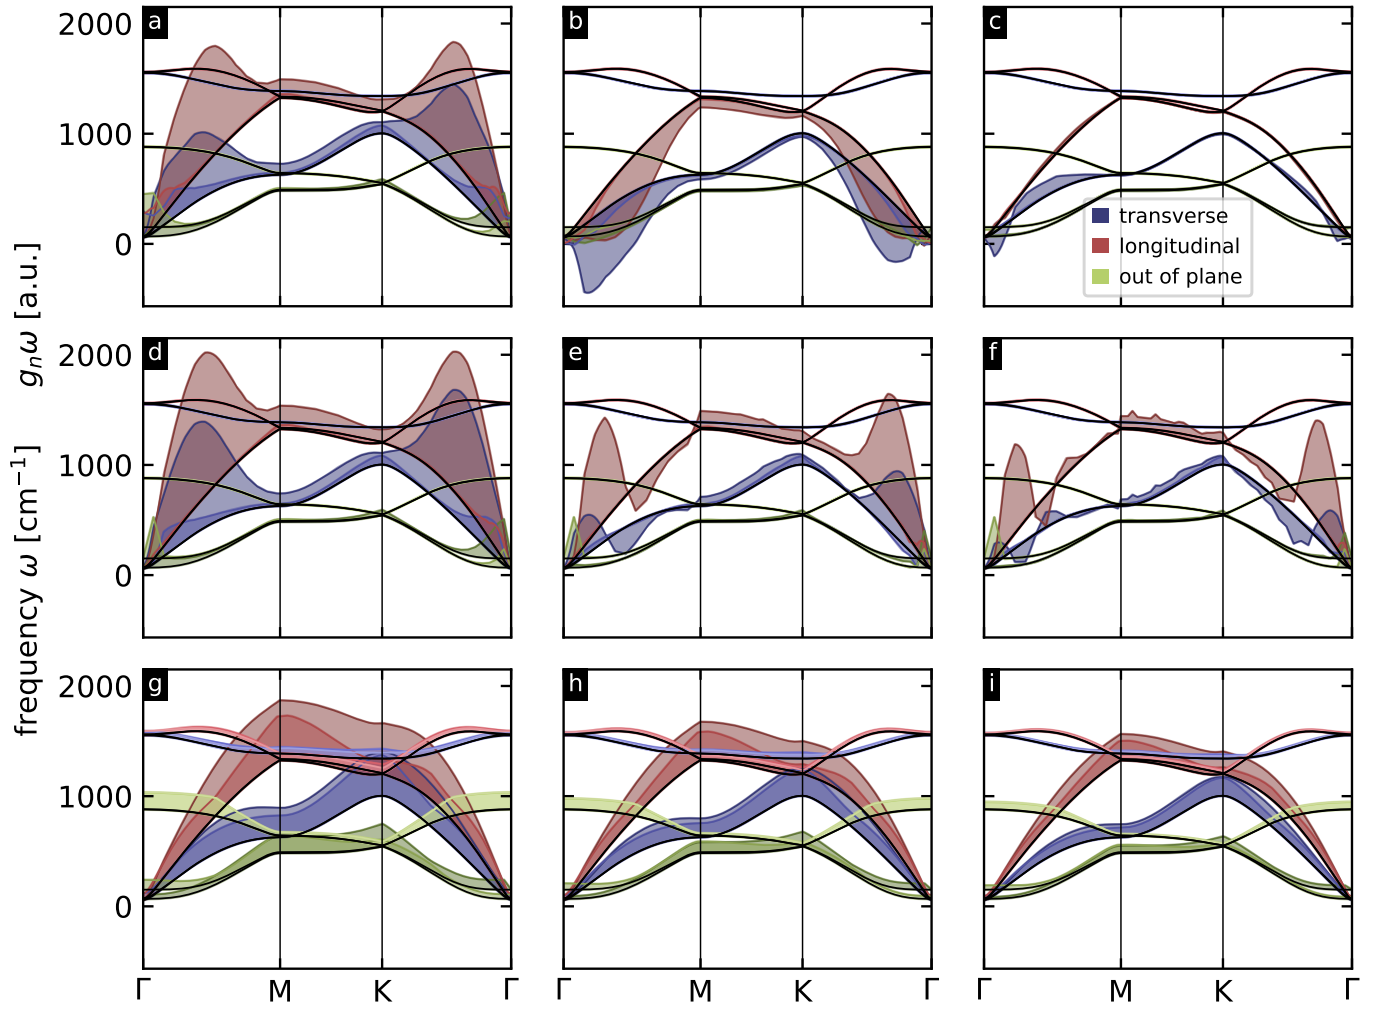

FIG. 2. (a)-(c) Graphite's phonon band structure along  $\overline{\Gamma\text{MK}\Gamma}$  in black solid lines. The shaded areas indicate the deviation of the energy stored  $g_n\omega$  in the modes from equilibrium for the three time steps 0.23 ns (a, d, g), 1.23 ns (b, e, h), and 1.95 ns (c, f, i). (a-c) present the data for the hydrodynamic case, (d-f) for the ballistic case, and (g-i) the diffusive case.
